# Supplementary material for: Electromagnetically induced transparency in inhomogeneously broadened divacancy defect ensembles in SiC
Source: arXiv:2203.09869 ancillary file (2022-03-18)
Supplement: Supplementary file 1 [file Supplementary_unmarked.pdf]

# Supplementary Information: Electromagnetically induced transparency in inhomogeneously broadened divacancy defect ensembles in SiC

Olger V. Zwier\*,<sup>1</sup> Tom Bosma\*,<sup>1</sup> Carmem M. Gilardoni,<sup>1</sup> Xu Yang,<sup>1</sup> Alexander  
R. Onur,<sup>1</sup> Takeshi Ohshima,<sup>2</sup> Nguyen T. Son,<sup>3</sup> and Caspar H. van der Wal<sup>1</sup>

<sup>1</sup>*Zernike Institute for Advanced Materials,  
University of Groningen, NL-9474AG Groningen, the Netherlands*

<sup>2</sup>*National Institutes for Quantum Science and Technology,  
1233 Watanuki, Takasaki, Gunma 370-1292, Japan*

<sup>3</sup>*Linköping University, Department of Physics,  
Chemistry and Biology, S-581 83 Linköping, Sweden*

(Dated: Version of January 19, 2022)

### A. Generation of a high divacancy concentration in 4H-SiC

The high concentration of divacancies in the 4H-SiC sample used in this work was generated by irradiating the sample with a 2 MeV electron beam with a dose of  $8 \times 10^{18} \text{ cm}^{-2}$ . Generally, this yields a broad range of lattice defects, such as carbon-vacancy, silicon-vacancy centers and divacancies. In order to optimize for the latter, the sample was annealed at  $750^\circ\text{C}$  for 15 minutes. This causes the carbon and silicon vacancies to diffuse leads to a higher concentration of divacancies since these are more stable. The sample was originally semi-insulating, with estimated concentrations of N and B on the order of  $7 \times 10^{15}$  and  $7 \times 10^{15} \text{ cm}^{-3}$ , respectively. The additional defects created during the irradiation process modify the Fermi level of this sample. Optically-detected bulk EPR (electron paramagnetic resonance) characterization at the growth lab showed that after annealing the Fermi level was pinned at 1.4 eV below the conduction band minimum, which corresponds to having the majority of the divacancies in their neutral charge state for the sample in dark equilibrium conditions.

### B. Measuring probe-beam absorption

As mentioned in the main text, all reported absorption traces are exclusively from probe absorption. The probe beam is separated from the control and repump beams by means of spatial separation: The beams cross each other in one point within the sample at angles below  $5^\circ$  (see Fig. S1). After transmission through the sample the probe beam passes through a 1000 nm long-pass filter to filter out any stray repump-beam radiation. Next it passes through a series of irises to filter out any stray control-beam radiation. Finally, it is captured by an InGaAs photodetector. All three beams are focused onto the sample by a lens outside the cryostat, with focal length 15 cm. We determine that the beams have a diameter of approximately  $70 \mu\text{m}$  at the sample. Their Rayleigh length is on the order of the sample length (2 mm), such that the spot size is approximately constant throughout the sample. Considering this spot size, the length of the sample and the  $< 5^\circ$  angle between control and probe beams, we conclude that the beams overlap significantly throughout the sample.

To increase the signal-to-noise ratio of the absorption measurements we implement a

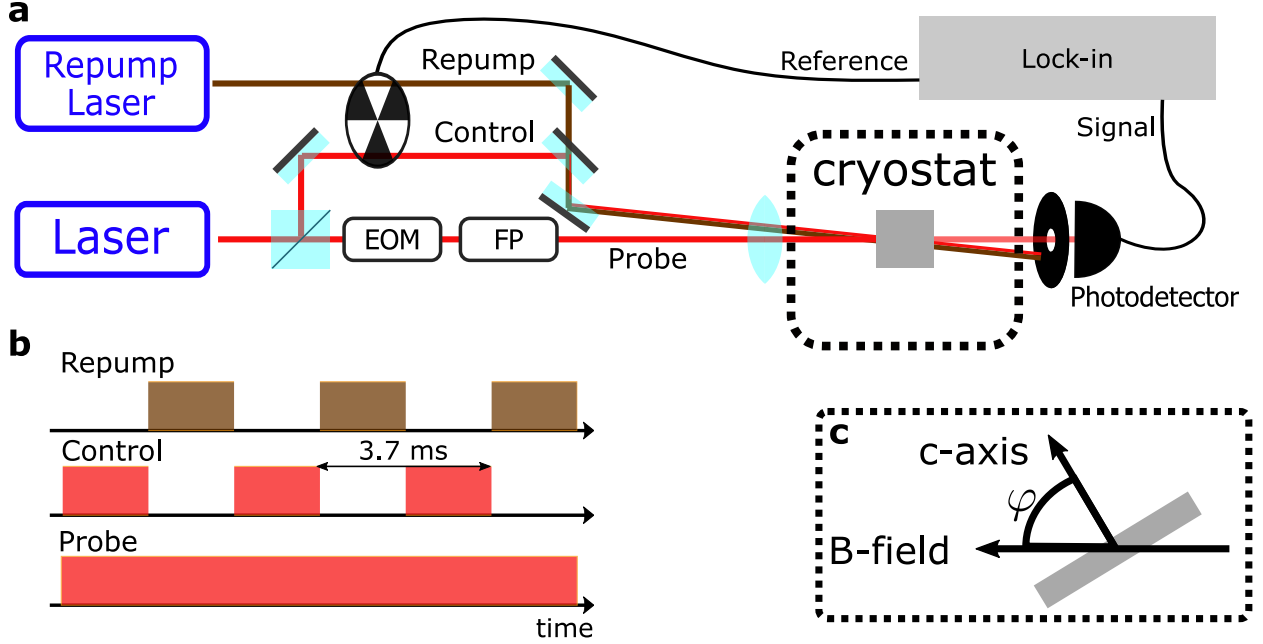

FIG. S1. **Measurement setup and pulse sequence.** **a)** Measurement setup. Both control and probe beams are created from a common laser. The probe beam is detuned from the control beam by an electro-optical modulator (EOM), and selected from additional sidebands by a Fabry-Pérot filter (FP). Both beams overlap inside the sample and the control beam is blocked by a series of irises, such that only the transmitted probe beam is detected at the photodetector. The control beam is modulated in time by a chopper. This time-modulation is used to extract the signal from simultaneous interaction with the control and probe beams using a lock-in amplifier. Additionally, we also use a repump laser (see text for details) to reinitialize the original charge configuration of the divacancies. This repump beam is also modulated by the chopper, but out of phase with respect to the control beam. Thus, whenever the control beam is on, the repump is off, as shown in the schematic representation of the pulse sequence (**b**). **c)** Magnetic field configuration inside of the cryostat. The field is applied at an angle  $\varphi$  with respect to the crystal c-axis.

cross-modulation method. Here, the control beam passes through a chopper wheel at 270 Hz prior to entering the sample. If the control beam is blocked by the chopper, the ensemble of divacancies is not optimally prepared in the  $|g_1\rangle$  state (see Fig. 1(c)), thus the probe-beam will be absorbed less. Conversely, if the control beam passes through the chopper freely, the population will be well prepared for probe absorption and the transmission of the probe beam will drop. In order to extract this 270 Hz modulation, the InGaAs photodetector signal is fed to a lock-in amplifier. The resulting signal (lock-in R) now exclusively represents probe-beam absorption.

Additionally, a 770 nm pulsed 10 mW repump laser (150 fs pulses, 80 MHz repetition rate, and beam diameter of approximately 100  $\mu\text{m}$  inside the sample) is present to counter

bleaching of the optical signal due to charge-state switching of the divacancies. This beam passes through the same chopper wheel as the probe beam and the alignment is tuned to have the on-off cycles of both beams in anti phase with each other. This way the influence of the repump beam on the coherence is strongly reduced when EIT is established. The divacancy can be repumped into its neutral charge state via band-gap excitation<sup>1</sup> or due to optical pumping of the charged defects into the phonon-sideband of their optically excited state<sup>2</sup>. The 770 nm laser does the latter. We observe that repumping is optimal for this wavelength, but works in general for a broad range of repump laser energies. We used a pulsed laser due to availability in our lab, but this is not a requirement for effective repumping.

### C. Pumping schemes for TLAF lines

We relate the two-laser absorption features (TLAF) depicted in Fig. 2(a) in the main text to pumping schemes in a six-level system by solving the ground and excited-state Hamiltonian for the energy eigenvalues. We have for the ground (excited) state Hamiltonian  $H_{g(e)}$

$$H_{g(e)} = g_{g(e)}\mu_B\mathbf{B} \cdot \mathbf{S} + \hbar D_{g(e)}S_z^2, \quad (1)$$

where we use  $D_g = 1.3$  GHz and  $D_e = 0.5$  GHz, as was found in<sup>3</sup>. For the ground (excited) state we set  $g_{g(e)} = 2$ . It is assumed that both the ground and excited state are  $S = 1$  triplets. Fig. S2a shows the energy splittings of the ground and excited-state spin sublevels. In total nine different optical transitions are possible between the ground and excited states. Their frequencies relative to the zero-phonon line are depicted in Fig. S2b, grouped per ground-state level by color. It can be seen that beyond 30 mT two transition pairs overlap for a broad range of magnetic field values. Below 30 mT just one pair of transitions overlaps: the  $|g_2\rangle - |e_2\rangle$  and  $|g_3\rangle - |e_3\rangle$  transitions (control laser transitions for  $\Lambda_1$  in Fig. 1(c) in the main text). The other pair consists of the  $|g_2\rangle - |e_1\rangle$  and  $|g_3\rangle - |e_2\rangle$  transitions (control laser transitions for  $\Lambda_2$  in Fig. 1(c) in the main text).

From these transitions we can find the detunings and magnetic field magnitudes at which to expect TLAF features. These are plotted in Fig. S2c for the TLAFs from Fig. 2a in the main text. We can relate the L<sub>1</sub>-L<sub>3</sub> features to the pumping schemes depicted in Fig. S3a-c. Note that, in the case of negative detuning, the probe and control lasers are effectively swapped. L<sub>1</sub> and L<sub>2</sub> both have a unique pumping scheme. The L<sub>3</sub> line may be caused by three different pumping schemes that lie closely together, one occurs at positive detuning, the other two at negative detuning. All these pumping schemes for  $\Lambda_3$  still allow for optical spin pumping into  $|g_1\rangle$  as no transition is driven from that level. This explains why that line shows up dimmer in Fig 2a and why we were unable to observe an EIT dip in its TLAF.

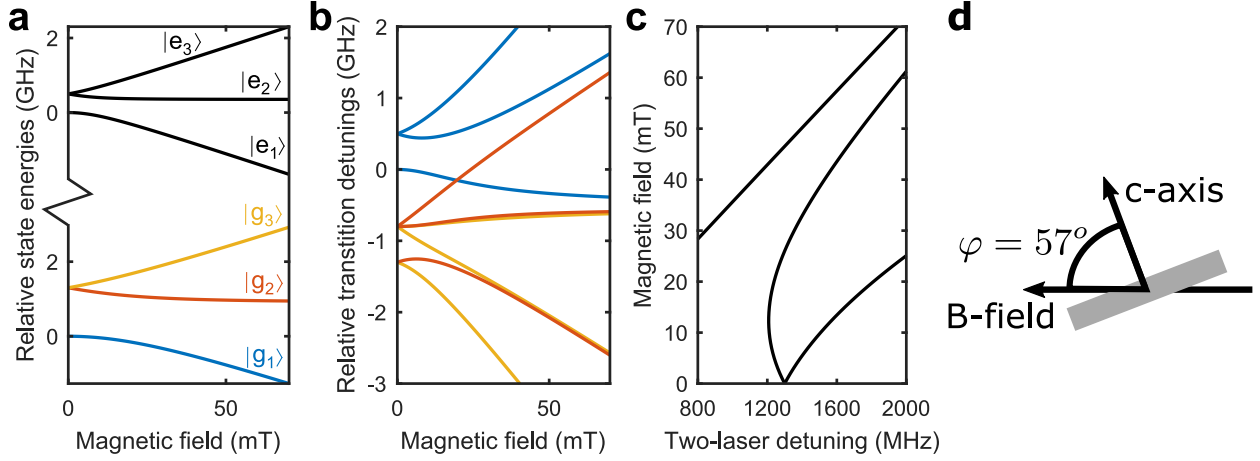

FIG. S2. **Level splittings and transition energies.** **a)** Energy level splittings versus magnetic field for the divacancy ground and excited-state sublevels. Energies for the ground (excited) state are relative to  $|g_1\rangle$  ( $|e_1\rangle$ ) **b)** Transition energies for the nine possible transitions between the ground and excited-state sublevels. The blue, orange, yellow lines correspond to transitions from the  $|g_1\rangle$ ,  $|g_2\rangle$ ,  $|g_3\rangle$  ground-state levels, respectively. Frequencies are relative to the  $|g_1\rangle - |e_1\rangle$  transition frequency **c)** Magnetic field and detuning dependence of several TLAFs obtained from combining transitions in **b)**. **d)** Magnetic field configuration, at an angle of  $57^\circ$  with respect to the crystal c-axis.

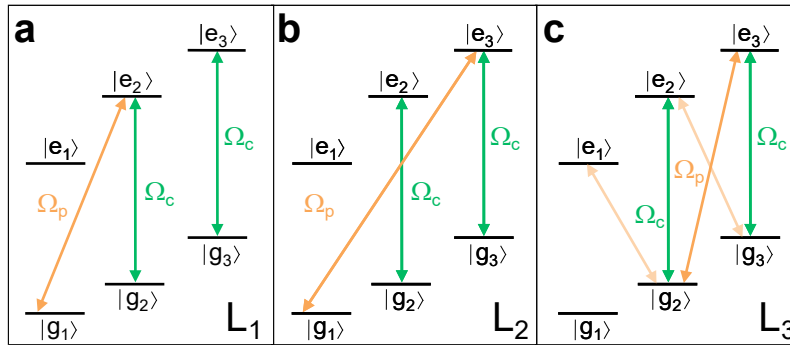

FIG. S3. **Pumping schemes for the observed TLAFs.** **a-c)** Pumping schemes for the  $L_1$ - $L_3$  features in Fig. S2c, respectively. Three different schemes are responsible of  $L_3$ , the opaque orange probe-beam transition occurs at positive detuning, the two translucent orange probe-beam transitions occur at negative detuning.

#### D. Density matrix for three-level system

We derive the density matrix  $\rho$  for a three-level system by using the master equation in Lindblad form

$$\dot{\rho} = -\frac{i}{\hbar} [H, \rho] + \mathcal{L}(\rho), \quad (2)$$

where  $H$  represents the Hamiltonian of the system and  $\mathcal{L}(\rho)$  the Lindblad superoperator containing the decay and dephasing terms of the system. Figure S4 shows the three-level system with the relevant laser couplings at hand.

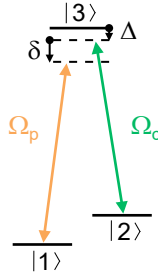

FIG. S4. **Three-level system for master equation.** This three-level systems with laser couplings for the probe and control laser is used as an example for the derivation of the density matrix from the master equation in Lindblad form. The control-laser detuning  $\Delta$  from resonance with the  $|2\rangle - |3\rangle$  transition and the detuning  $\delta$  from two-photon resonance are depicted.

We first derive the Hamiltonian  $H$  for this system, we get

$$H = H_0 + V, \quad (3)$$

where  $H_0$  represents the Hamiltonian of the unperturbed system and  $V$  the perturbations from the optical driving fields. We get

$$\mu = \begin{pmatrix} \hbar\omega_1 & 0 & 0 \\ 0 & \hbar\omega_2 & 0 \\ 0 & 0 & \hbar\omega_3 \end{pmatrix}, \quad (4)$$

where  $\hbar\omega_i$  represents the energy for state  $i$ . For the perturbation  $V$  we use the electric dipole approximation to get<sup>4</sup>

$$V = -\mu E, \quad (5)$$

where  $E$  is the applied optical field and  $\mu$  the dipole operator. We have dropped the vector notation by assuming that the optical electric fields are always perfectly aligned with the dipole moments. The field  $E$  with an applied probe and control laser is

$$E = \frac{1}{2} [E_p e^{i\omega_p t} + E_c e^{i\omega_c t} + c.c.], \quad (6)$$

with  $E_p$  ( $E_c$ ) the electric field amplitude and  $\omega_p$  ( $\omega_c$ ) the frequency of the probe (control) field. For the dipole operator  $\mu$  we ignore the static dipoles and the transition dipole for the  $|1\rangle - |2\rangle$  transition (and vice versa), as it is far off resonance. We get

$$\mu = \begin{pmatrix} 0 & 0 & \mu_{13} \\ 0 & 0 & \mu_{23} \\ \mu_{31} & \mu_{32} & 0 \end{pmatrix}. \quad (7)$$

Now we can construct the full Hamiltonian  $H$ . We can reduce the number of driving terms for the perturbation part by applying the rotating wave approximation (RWA). For this, we first need to convert to the interaction picture by performing the unitary transformation  $H' = U H U^\dagger$  with

$$U = e^{iH_0 t/\hbar} = \begin{pmatrix} e^{i\omega_1 t} & 0 & 0 \\ 0 & e^{i\omega_2 t} & 0 \\ 0 & 0 & e^{i\omega_3 t} \end{pmatrix}. \quad (8)$$

Since we have  $\omega_p \approx \omega_3 - \omega_1$  and  $\omega_c \approx \omega_3 - \omega_2$ , some off-diagonal terms in  $H$  evolve far slower than others. The fast terms become irrelevant in this picture. Upon ignoring these terms and rotating back to the Schrödinger picture we get

$$H = \begin{pmatrix} \hbar\omega_1 & 0 & -\frac{\mu_{13}E_p}{2}e^{i\omega_p t} \\ 0 & \hbar\omega_2 & -\frac{\mu_{23}E_c}{2}e^{i\omega_c t} \\ -\frac{\mu_{32}E_p}{2}e^{-i\omega_p t} & -\frac{\mu_{31}E_c}{2}e^{-i\omega_c t} & \hbar\omega_3 \end{pmatrix}. \quad (9)$$

For compactness, we substitute the Rabi frequencies  $\Omega_p = \frac{\mu_{13}E_p}{\hbar} = \frac{\mu_{31}E_p}{\hbar}$  and  $\Omega_c = \frac{\mu_{23}E_c}{\hbar} = \frac{\mu_{32}E_c}{\hbar}$ . In general, both the electric field amplitude and the transition dipole moments are

here complex numbers that take into consideration also the phase of the oscillating electric fields and driven dipoles, respectively. This is accounted for when formulating the CPT state as (for the case of ideal spin coherence<sup>5</sup>)  $|\Psi_{CPT}\rangle \propto \Omega_c |1\rangle - \Omega_p |2\rangle$ , and in steady state the system settles in this dark state for two-photon resonance. However, the systems considered here are driven adiabatically, that is, any change in the phase of the driving fields is slower than the intrinsic dynamics and coherences of the quantum system. In this case, the phase in the electric field is quickly counteracted by a phase in the driven quantum system, leading to Rabi frequencies that can be taken as real without loss of generality. For the interacting Hamiltonian above, we get

$$H = \hbar \begin{pmatrix} \omega_1 & 0 & -\frac{\Omega_p}{2} e^{i\omega_p t} \\ 0 & \omega_2 & -\frac{\Omega_c}{2} e^{i\omega_c t} \\ -\frac{\Omega_p}{2} e^{-i\omega_p t} & -\frac{\Omega_c}{2} e^{-i\omega_c t} & \omega_3 \end{pmatrix}. \quad (10)$$

In order to solve the master equation (Eq. 3) we have to get rid of the oscillating terms. This can be done by performing another unitary transformation, converting to a frame that rotates along with these oscillating terms. Let's call the density operator in this rotating frame  $\sigma$  and relate it to  $\rho$  by  $\rho = R\sigma R^\dagger$  a proper choice for  $R$  is then a diagonal matrix where

$$R_{ii} = \begin{cases} e^{i\omega_k} & \text{if only one field } \omega_k \text{ couples to level } i \\ 1 & \text{otherwise} \end{cases}. \quad (11)$$

For our three-level system we get

$$\begin{pmatrix} e^{i\omega_p t} & 0 & 0 \\ 0 & e^{i\omega_c t} & 0 \\ 0 & 0 & 1 \end{pmatrix}. \quad (12)$$

The master equation (Eq. 3) now becomes (ignoring the Lindblad superoperator for now)

$$\left( \dot{R}\sigma R^\dagger + R\dot{\sigma} R^\dagger + R\sigma \dot{R}^\dagger \right) = -\frac{i}{\hbar} [H, R\sigma R^\dagger]. \quad (13)$$

This will yield only static terms in the relation between  $\dot{\sigma}$  and  $\sigma$ .

Before we can start solving the master equation, we still need the Lindblad superoperator  $\mathcal{L}(\sigma)$ , which contains the decay and dephasing terms. In this rotating frame it can be defined as follows<sup>4,5</sup>

$$[\mathcal{L}(\sigma)]_{ij} = \begin{cases} \Gamma_{ki}\sigma_{kk} - \Gamma_{ik}\sigma_{ii} & \text{for } i = j \\ -\left[\frac{1}{2}(\Gamma_{ik} + \Gamma_{jk}) + \gamma_i + \gamma_j\right]\sigma_{ij} & \text{for } i \neq j \end{cases}, \quad (14)$$

where  $\Gamma_{ij}$  represents the decay rate from level  $|i\rangle$  to  $|j\rangle$ ,  $\gamma_i$  and the dephasing rate for level  $|i\rangle$ . Note that the Einstein summation convention is used here.

Now we can write the components of  $\dot{\sigma}$  as a system of nine coupled equations like  $\dot{\sigma} = M\sigma$ . We set  $\Gamma_{12} = \Gamma_{21} = \Gamma_g \neq 0$  and  $\Gamma_{31} = \Gamma_{32} = \Gamma_e \neq 0$ , all other decay terms are set to zero. For the dephasing terms we set  $\gamma_1 = 0$  to consider all phases relative to state  $|1\rangle$ . Furthermore, since in our system the decay rate from the excited state is several orders of magnitude larger than the dephasing rate  $\gamma_3$ , we ignore it by setting  $\gamma_3 = 0$ . Additionally, we substitute the control-laser detuning  $\Delta = \omega_3 - \omega_2 - \omega_c$  and the probe-laser detuning  $\delta + \Delta = \omega_3 - \omega_1 - \omega_p$ . Now we get for our three level system

$$\begin{bmatrix} \dot{\sigma}_{11} \\ \dot{\sigma}_{12} \\ \dot{\sigma}_{13} \\ \dot{\sigma}_{21} \\ \dot{\sigma}_{22} \\ \dot{\sigma}_{23} \\ \dot{\sigma}_{31} \\ \dot{\sigma}_{32} \\ \dot{\sigma}_{33} \end{bmatrix} = \begin{pmatrix} -\Gamma_g & 0 & i\frac{\Omega_p}{2} & 0 & \Gamma_g & 0 & -i\frac{\Omega_p}{2} & 0 & \Gamma_e \\ 0 & -i\delta - \Gamma_g - \gamma_2 & i\frac{\Omega_c}{2} & 0 & 0 & 0 & 0 & -i\frac{\Omega_p}{2} & 0 \\ i\frac{\Omega_p}{2} & i\frac{\Omega_c}{2} & -i(\Delta + \delta) - \Gamma_e - \frac{\Gamma_g}{2} & 0 & 0 & 0 & 0 & 0 & -i\frac{\Omega_p}{2} \\ 0 & 0 & 0 & i\delta - \Gamma_g - \gamma_2 & 0 & i\frac{\Omega_p}{2} & -i\frac{\Omega_c}{2} & 0 & 0 \\ \Gamma_g & 0 & 0 & 0 & -\Gamma_g & i\frac{\Omega_c}{2} & 0 & -i\frac{\Omega_c}{2} & \Gamma_e \\ 0 & 0 & 0 & i\frac{\Omega_p}{2} & i\frac{\Omega_c}{2} & -i\Delta - \Gamma_e - \frac{\Gamma_g}{2} - \gamma_2 & 0 & 0 & -i\frac{\Omega_c}{2} \\ -i\frac{\Omega_p}{2} & 0 & 0 & -i\frac{\Omega_c}{2} & 0 & 0 & i(\Delta + \delta) - \Gamma_e - \frac{\Gamma_g}{2} & 0 & i\frac{\Omega_p}{2} \\ 0 & -i\frac{\Omega_p}{2} & 0 & 0 & -i\frac{\Omega_c}{2} & 0 & 0 & i\Delta - \Gamma_e - \frac{\Gamma_g}{2} - \gamma_2 & i\frac{\Omega_c}{2} \\ 0 & 0 & -i\frac{\Omega_p}{2} & 0 & 0 & -i\frac{\Omega_c}{2} & i\frac{\Omega_p}{2} & i\frac{\Omega_c}{2} & -2\Gamma_e \end{pmatrix} \begin{bmatrix} \sigma_{11} \\ \sigma_{12} \\ \sigma_{13} \\ \sigma_{21} \\ \sigma_{22} \\ \sigma_{23} \\ \sigma_{31} \\ \sigma_{32} \\ \sigma_{33} \end{bmatrix} .$$

The  $\dot{\sigma} = M\sigma$  system of equations can be solved if we define the total population in the system to be unity

$$\sigma_{11} + \sigma_{22} + \sigma_{33} = 1. \quad (15)$$

The material susceptibility to the probe laser  $\chi(\omega_p)$ , and thus its absorption coefficient, is proportional to the  $\sigma_{13}$  component of the density matrix<sup>5</sup>.

### E. Fitting routine

In similar fashion as in section D we derived a system of equations based on the master equation for the five-level system and laser couplings from figure 5(a) in the main text. To include the inhomogeneity of the transition frequency we calculated the probe absorption for a range of single-laser detuning  $\Delta$  values. The total ensemble probe absorption was computed as a weighted sum, determined by a Gaussian distribution of  $\Delta$  with a FWHM width of 140 GHz. We also considered the inhomogeneity of the optical intensity throughout the laser spot in our model. Perfect Gaussian beams and perfect overlap were assumed. All six double EIT traces from the power dependence measurement of Fig. 5(c) in the main text were fit simultaneously to the model with a least-squares method. This way we obtained unique values for the transition dipole moments. For fitting the temperature dependent traces in Fig. 5(d) the transition dipole moments were kept fixed to these values.

### F. Absorption background in two-laser spectroscopy

In order to understand the broad background absorption (that only occurs outside the spectral range of the EIT dip), which appears together with the linear TLAF absorption peak and the EIT dip in Figure 3a of the main text, we model the probe absorption of an inhomogeneous ensemble of three-level systems while varying both the ratio between control and probe beam powers and the ground-state relaxation  $\Gamma_g$  (Fig. S5a-d). This background arises due to probe absorption by detuned subensembles, that is, subensembles with large  $\Delta$  detunings. For these defects, the control beam (driving transitions from state  $|g_2\rangle$  in Fig. S3a) is continuously detuned from the optical transition, while the probe beam (which drives transitions from state  $|g_1\rangle$ ) has its frequency scanned. Any steady-state effect that repopulates the state  $|g_1\rangle$  of these subensembles at large values of two-photon detuning  $\delta$

will be of importance for this background. There are two effects at play.

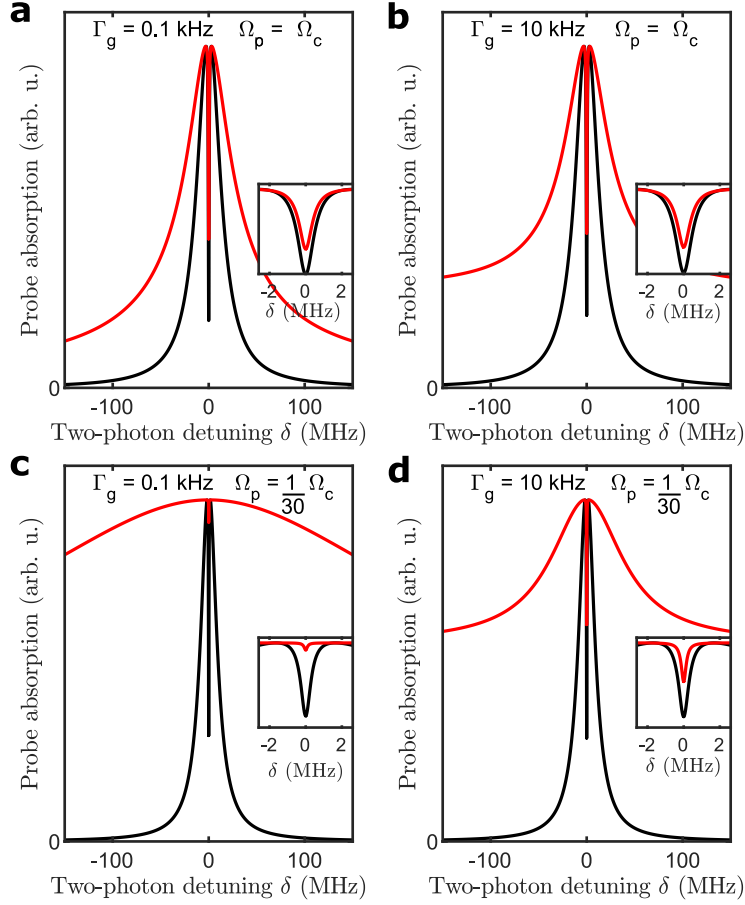

**FIG. S5. Background level in TLAf probe absorption for an inhomogeneous ensemble of three-level systems.** **a,b** Probe absorption versus two-photon detuning for systems driven by probe and control lasers with equal powers and **c,d** strongly asymmetric powers (control much stronger than probe). As in the main text, the black trace corresponds to the absorption of a homogeneous system with  $\Delta = 0$ , whereas the red trace corresponds to absorption of an inhomogeneous ensemble with broadening on the order of 100 GHz. For all plots we use the parameters as in Table I of the main text unless stated otherwise. To be clear, all plots have  $\Omega_c = 3 \times 10^6$  Hz, and  $\Omega_p$  and  $\Gamma_g$  vary as labeled.

First, after optical spin-pumping has reached steady-state, any spin-flip in the ground state will repopulate  $|g_1\rangle$ , and in turn cause probe absorption. This explains the increase in background level when comparing the red traces in Fig. S5a,d at the largest two-photon detunings. That is, here the level goes to that of single-laser probe absorption, and becomes very low for  $\Gamma_g < 1$  kHz.

Second, despite being far detuned, strong enough control beams can still lead to slow optical spin pumping. This effect causes the strong broadening of the TLAf feature as in

Fig. S5c, and this effect increases when reducing the rate  $\Gamma_g$ . These slow optical pumping effects can only take place if not disturbed by a spin-flip in the ground state, and become relatively important for the full TLA peak shape if also the optical pumping by the probe is weak (and note that the plots are normalized, and that this effect happens at an absolute scale this is a relatively weak level of probe absorption). We notice the resemblance between the modeled behavior of case (Fig. S5c) and the experimentally measured traces in Fig. 2d of the main text.

Finally, we note that this single-laser background absorption does not degrade the quality of the EIT dip, as demonstrated in Fig. S6. This plot is obtained for large control and probe Rabi frequencies ( $\Omega_c = \Omega_p = 15$  MHz). The trace corresponding to absorption by an inhomogeneous ensemble clearly shows a background absorption level that is non-zero. Nonetheless, the absorption at the EIT feature at  $\delta = 0$  goes to a value that is lower than this background absorption, and approaches zero for high control powers or slow ensemble dephasing times.

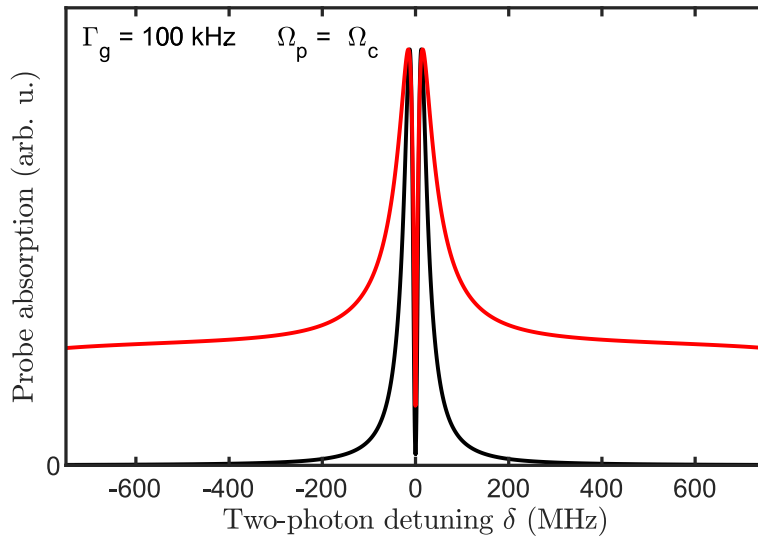

FIG. S6. **High driving powers and near-complete EIT.** Probe absorption versus two-laser detuning for systems driven by probe and control lasers with equal, large powers ( $\Omega_c = 15$  MHz), and with spin-dephasing time limited by the spin relaxation time  $\Gamma_g = 100$  kHz (increased to a higher value to give a larger background absorption), showing that the depth of the EIT feature is not limited by the background absorption level.

- 
- <sup>1</sup> Gary Wolfowicz, Christopher P Anderson, Andrew L Yeats, Samuel J Whiteley, Jens Niklas, Oleg G Poluektov, F Joseph Heremans, and David D Awschalom, “Optical charge state control of spin defects in 4H-SiC,” *Nat. Commun.* **8**, 1876 (2017).
- <sup>2</sup> O. V. Zwier, D. O’Shea, A. R. Onur, and C. H. van der Wal, “All-optical coherent population trapping with defect spin ensembles in silicon carbide,” *Sci. Rep.* **5**, 10931 (2015).
- <sup>3</sup> Olger V. Zwier, Zernike Institute PhD thesis series, ISSN 1570-1530 (University of Groningen, 2016).
- <sup>4</sup> Robert W Boyd, Daniel J Gauthier, Alexander L Gaeta, and Alan E Willner, “Maximum time delay achievable on propagation through a slow-light medium,” *Phys. Rev. A* **71**, 023801 (2005).
- <sup>5</sup> Michael Fleischhauer, Atac Imamoglu, and Jonathan P Marangos, “Electromagnetically induced transparency: Optics in coherent media,” *Rev. Mod. Phys.* **77**, 633 (2005).
